# Supplementary material for: Topology and spectral interconnectivities of higher-order multilayer networks
Source: arXiv:2305.05860 source file (2023-06-26)
Supplement: Supplementary file 1 [file SI_ATN_SCH_dist.tex]

%% SI fig : ATN SCH distributions
%%% SI: fig PCH 
\begin{figure}[!ht]
\begin{tabular}{ll}
Lufthansa to Ryanair & Lufthansa to Easyjet \\
 \includegraphics[width=0.3\textwidth]{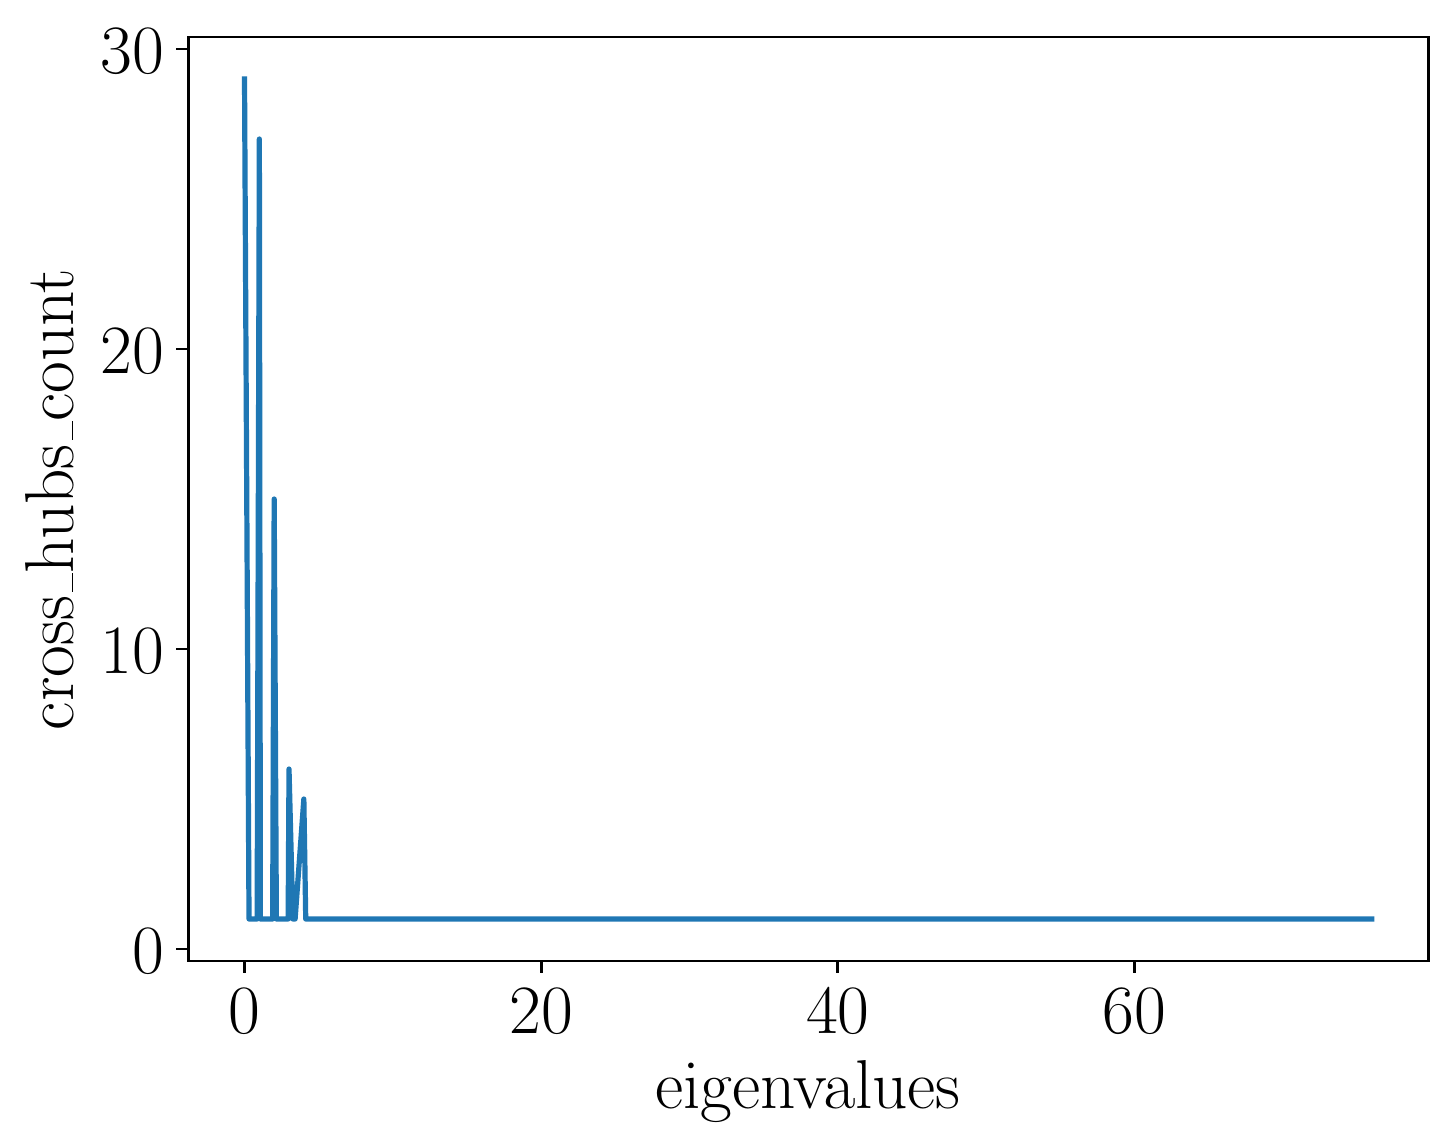} 
 &
  \includegraphics[width=0.3\textwidth]{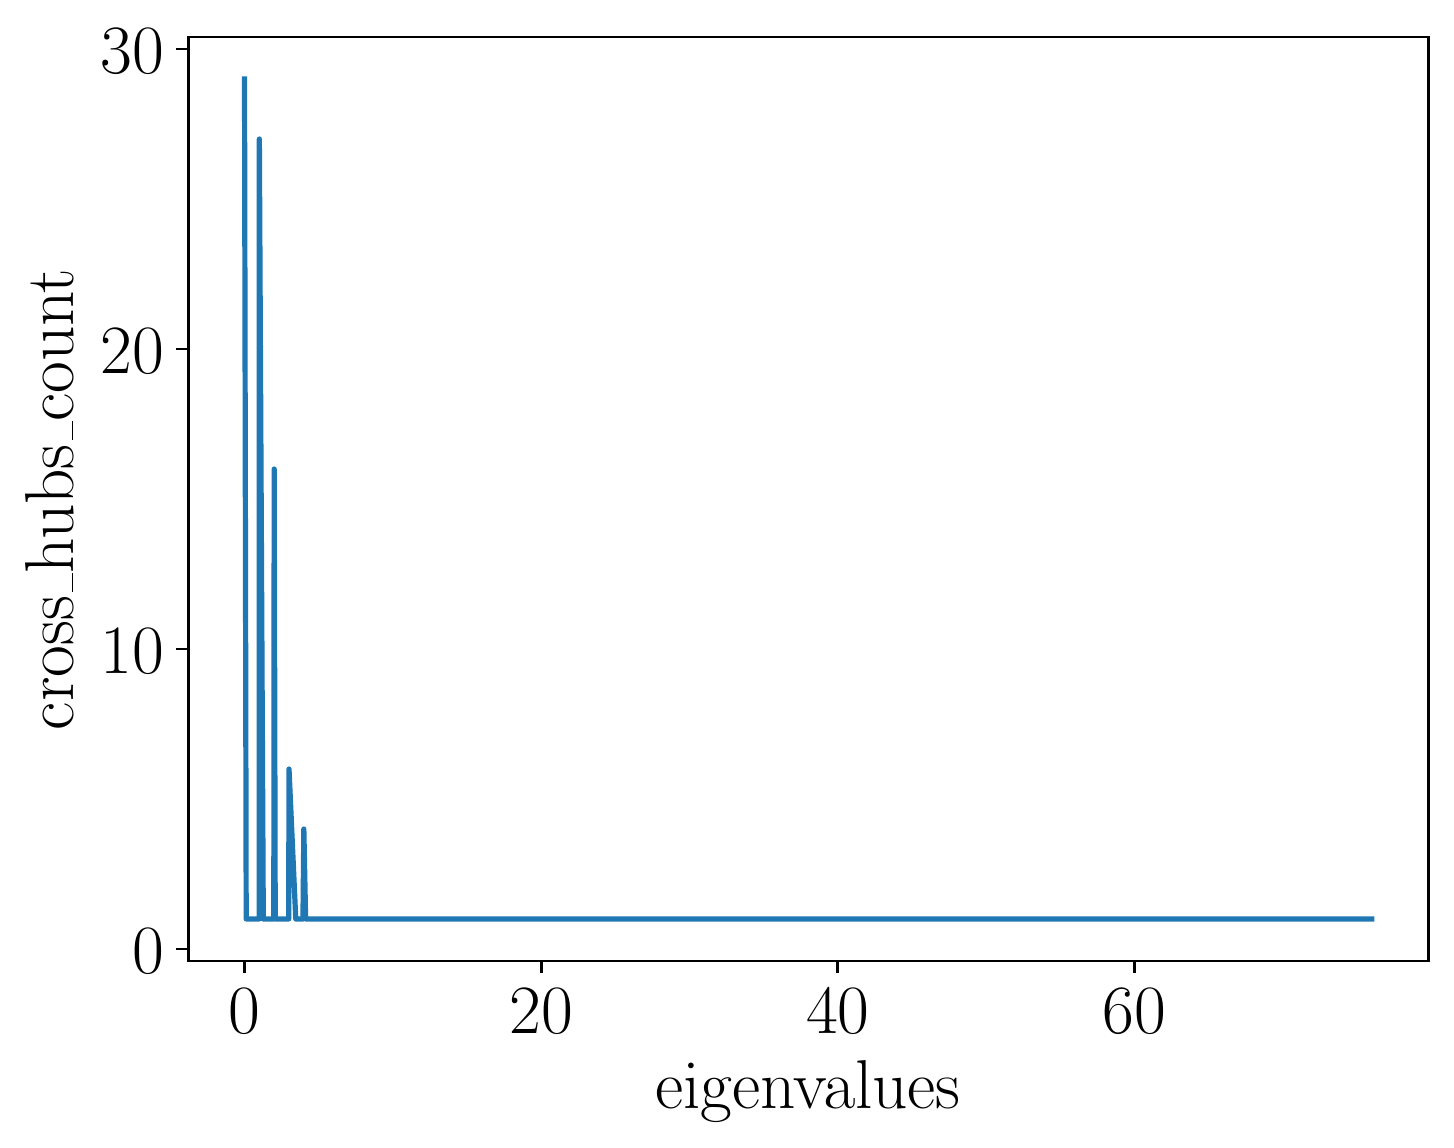}  \\
  Ryanair to Lufthansa & Rynair to Easyjet \\
    \includegraphics[width=0.3\textwidth]{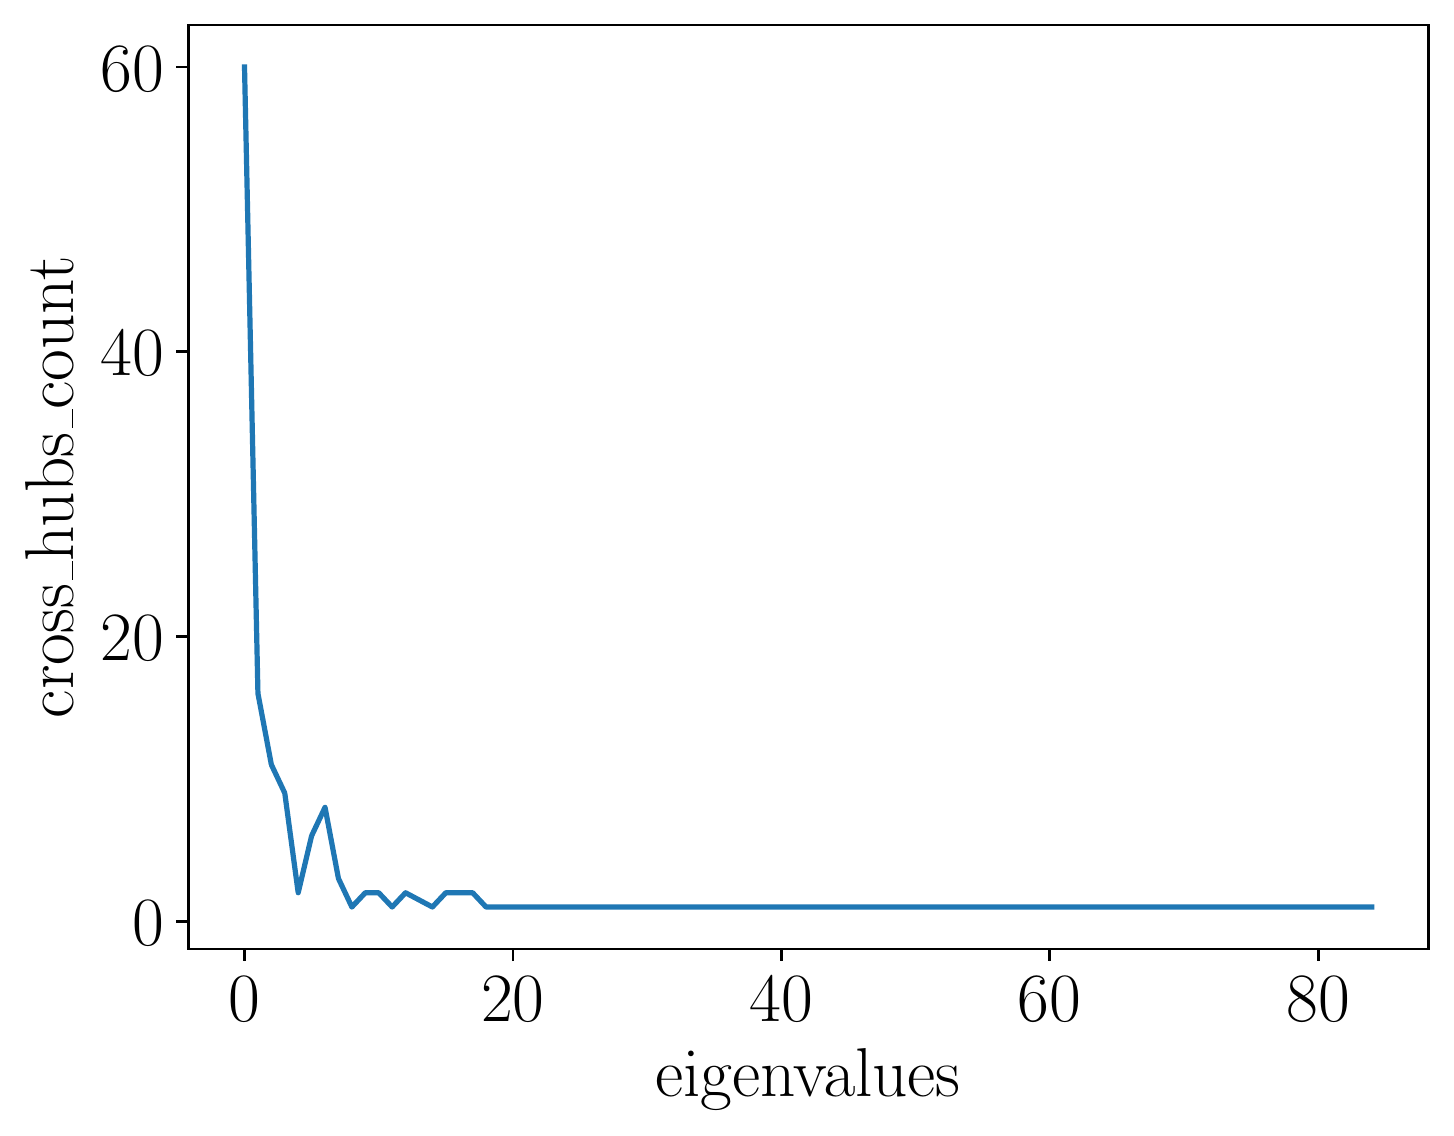}  
    &
    \includegraphics[width=0.3\textwidth]{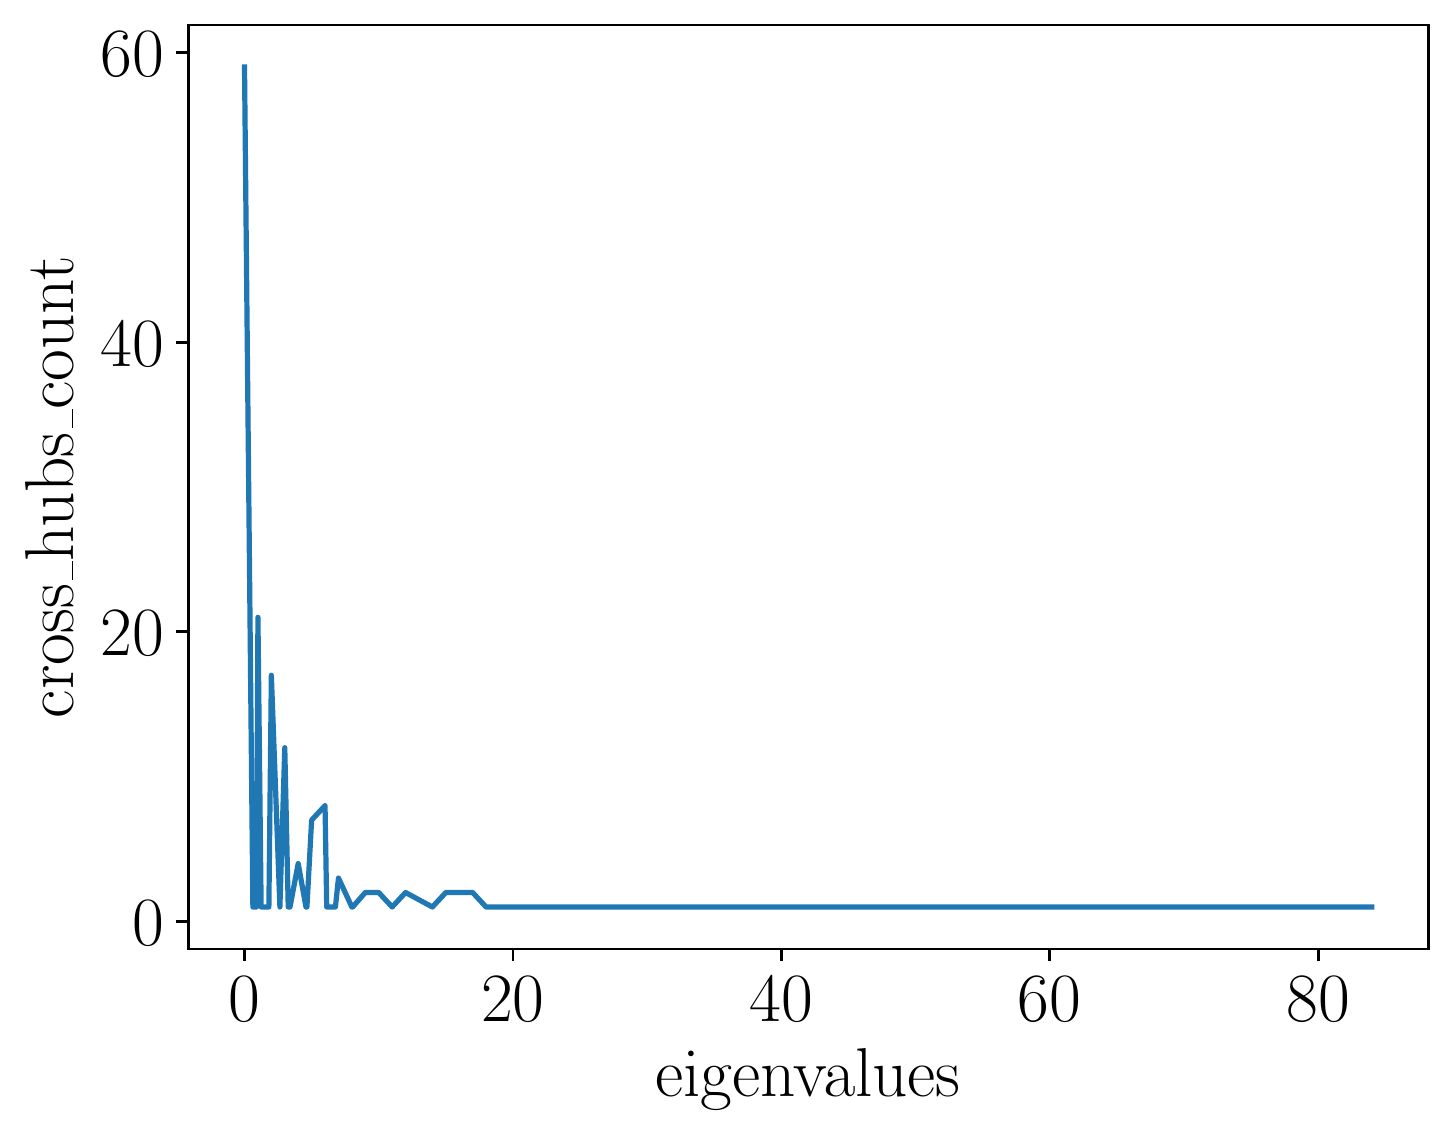} \\
 Easyjet to Lufthansa & Easyjet to Ryanair \\ 
  \includegraphics[width=0.3\textwidth]{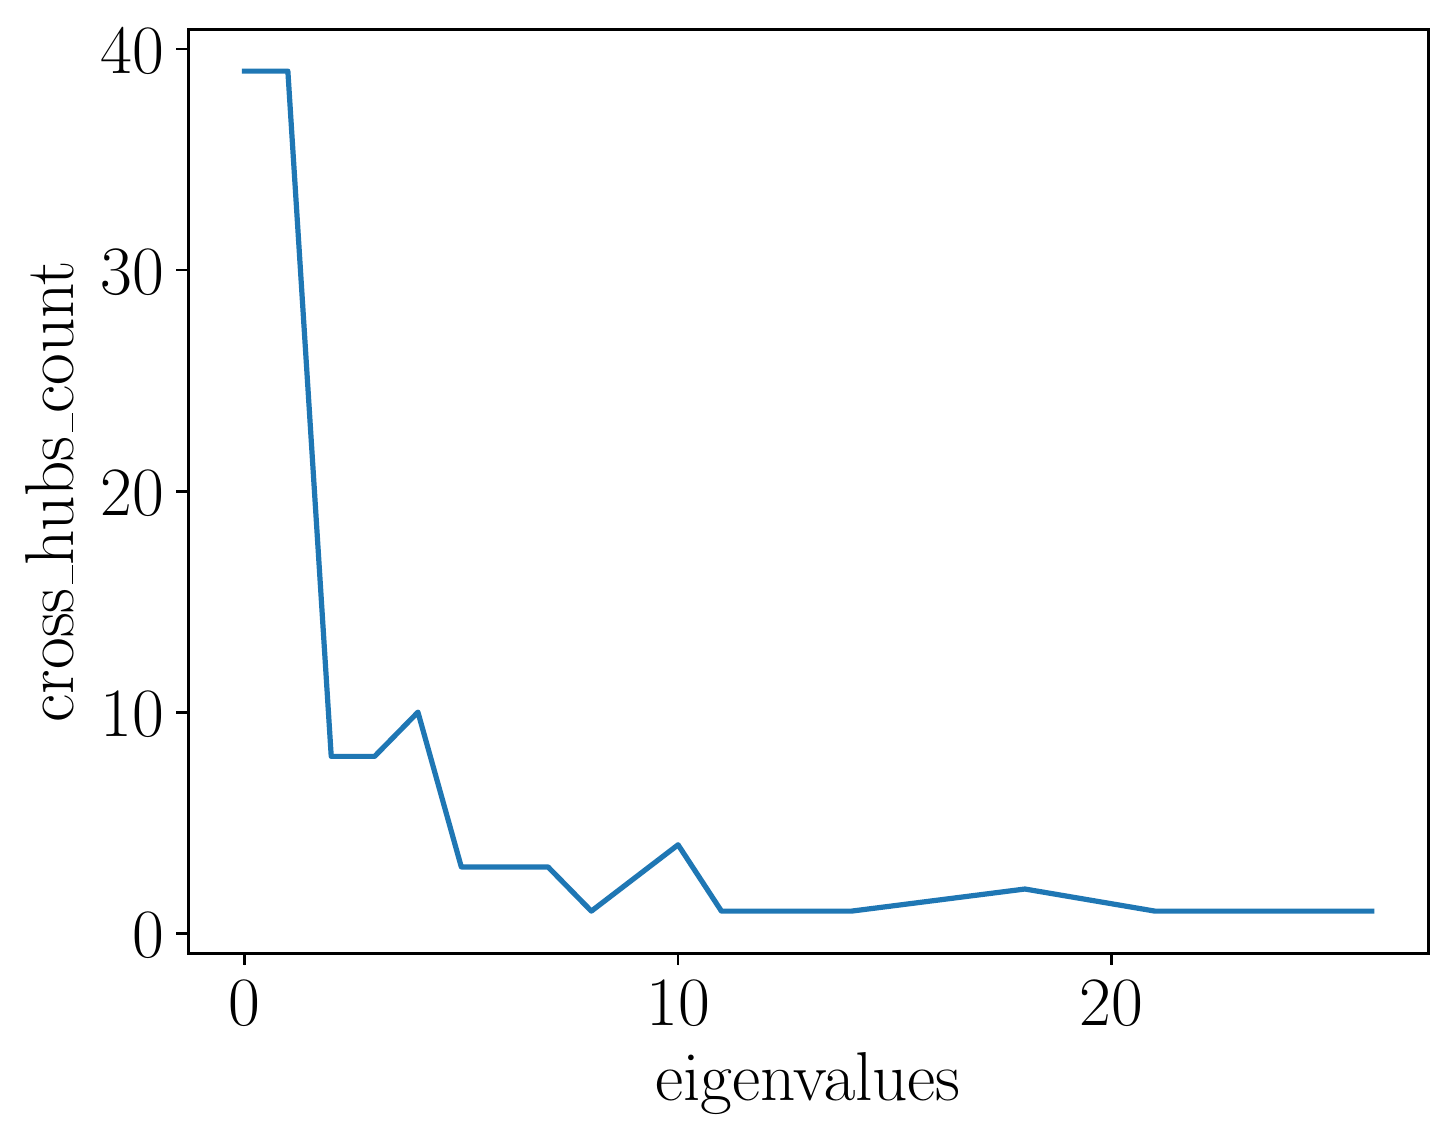}  
  &
    \includegraphics[width=0.3\textwidth]{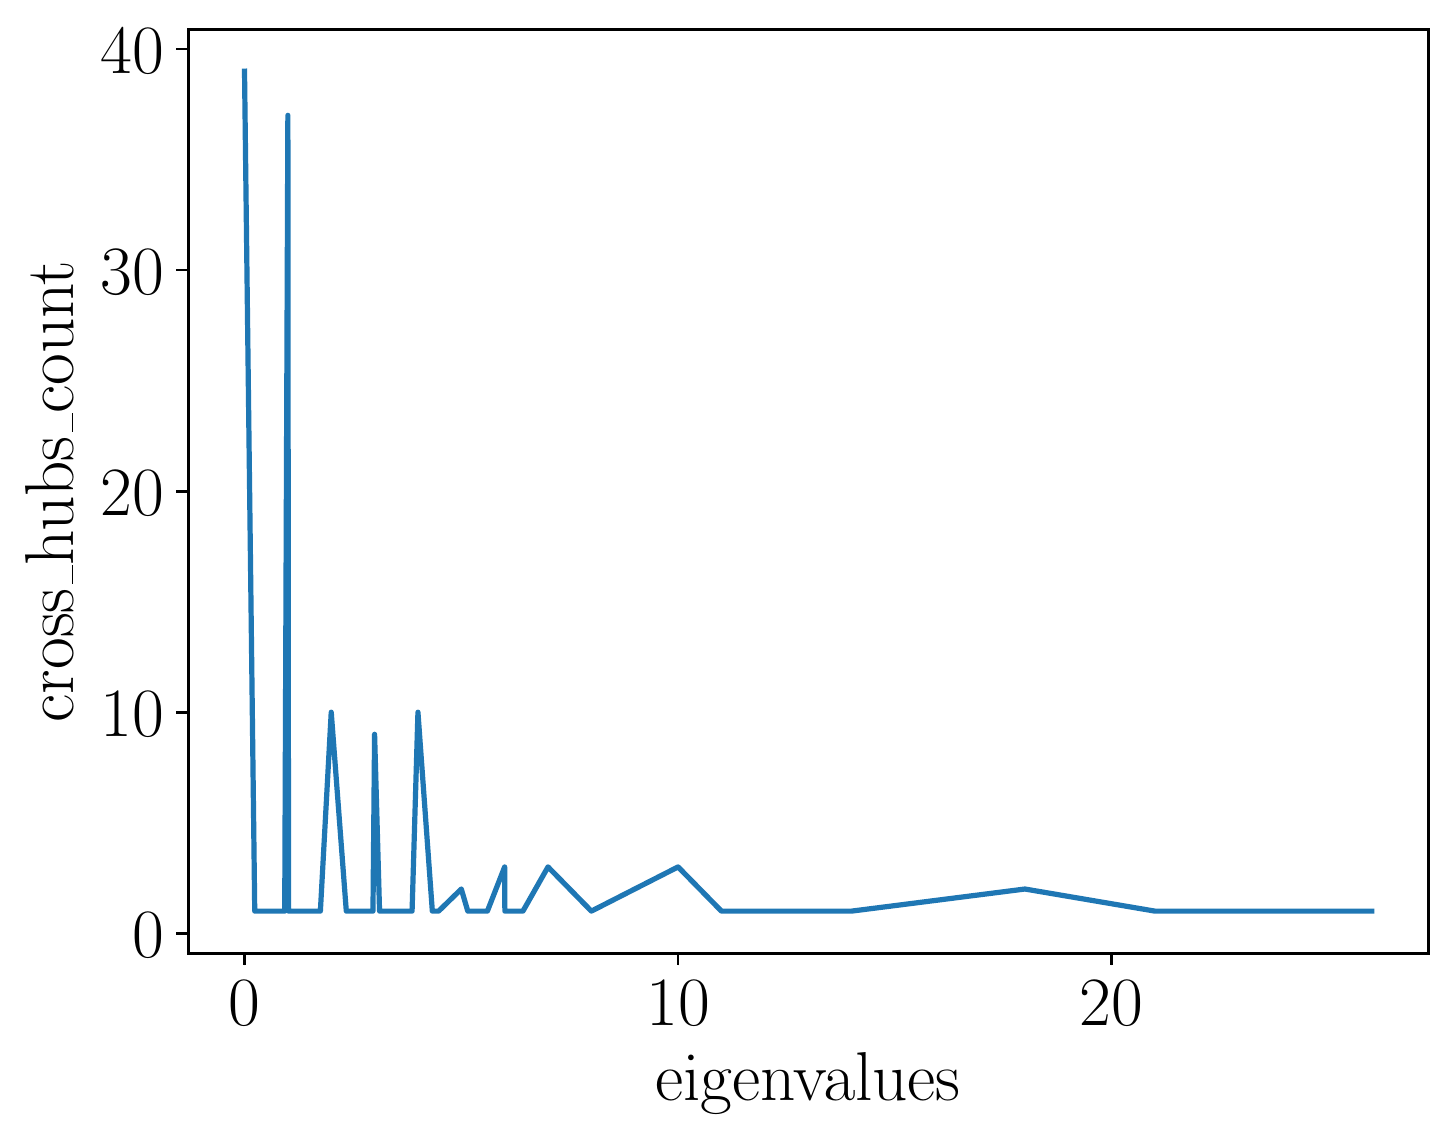}  

\end{tabular}
\caption{{\bf Spectral cross-hubs given by $\Lap{B}{0,0}$.} Variations of the number SCHs for the diffusion bicomplexes associated to the European ATN multiplex. The amount of SCHs tend to vary dramatically along the the smallest eigenvalues before it eventually stabilizes at a very low number.}
\label{fig:atn-SPB}
\end{figure}
