# Supplementary material for: Topology and spectral interconnectivities of higher-order multilayer networks
Source: arXiv:2305.05860 source file (2023-06-26)
Supplement: Supplementary file 3 [file SI_xLap_computations.tex]

%%%% SI: fig - xLap-computations
\begin{figure}[!ht]
\centering
\begin{tikzpicture}[scale=0.9]
%\tikzstyle{every node}=[font=\tiny]

%%%Layers 
%%%% V_1
\begin{scope}[on background layer,opacity=0.5]
\fill[gray!20] (0,0) -- (10,0) -- (8,2) node[midway,above, black] {$ \ V_1$} -- (1,2)  -- cycle;
%%%% V_2
\fill[red!20] (0,-3) -- (10,-3) -- (8,-1)  node[midway,above, black] {$ \ V_2$} -- (1,-1) -- cycle;
\end{scope}

%%% Vertices in V1 
\node[vertex] (u0) at (7,1.5) {};
\node at (7.4,1.5) {$v^1_0$};
\node[vertex] (u1) at (6,0.5) {};
\node at (6.6,0.5) {$v^1_1$};
\node[vertex] (u2) at (4,1.2) {};
\node at (4,1.6) {$u_2$};
\node[vertex] (u3) at (2,1.5) {};
\node at (1.6,1.5) {$v^1_3$};
\node[vertex] (u4) at (3,0.5) {};
\node at (2.6,0.5) {$v^1_4$};

%%% Vertices in V2
\node[vertex] (v0) at (7,-2.5) {};
\node at (7.4, -2.5) {$v^2_0$};
\node[vertex] (v1) at (6,-1.5) {};
\node at (5.6, -1.5) {$v^2_1$};
\node[vertex] (v2) at (5,-2.5) {};
\node at (5,-2.8) {$v^2_2$};
\node[vertex] (v3) at (3,-2) {};
\node at (3, -2.4) {$v^2_3$};

% %%% Crossimplices
\draw (u0) -- (u1) -- (u2) -- (u0);
\draw (u3) -- (u2) -- (u4);

\draw (v0) -- (v1) -- (v2) -- (v0);
\draw (v2) -- (v3);

\draw[dashed] (v0) -- (u1) -- (v1);
\draw[dashed] (u2) -- (v3) -- (u3);
\draw[dashed] (u4) -- (v3);
\draw[dashed] (u3) -- (v1) -- (u4);

%% Filling the triangles
\begin{scope}[on background layer]
\fill[purple!70, opacity=0.8] (u0.center) -- (u1.center) -- (u2.center) -- cycle;
\fill[yellow!70, opacity=0.8] (v0.center) -- (v1.center) -- (v2.center) -- cycle;
\end{scope}

\begin{scope}[on background layer]
\fill[blue!15, opacity=0.8] (u1.center) -- (v0.center) -- (v1.center) -- cycle;
\fill[green!40, opacity=0.8] (u2.center) -- (v3.center) -- (u4.center) -- cycle;
\fill[green!40, opacity=0.6] (u2.center) -- (v3.center) -- (u3.center) -- cycle;
\end{scope}

\end{tikzpicture}

\caption{A crossimplicial bicomplex of dimension $3$.}
\label{fig:calculations-laplacians}
\end{figure}
